# Supplementary material for: Transcoders Find Interpretable LLM Feature Circuits
Source: arXiv:2406.11944 source file (2024-11-06)
Supplement: Supplementary file 1 [file appendix.tex]

\section{Appendix}

Hello world
